# Supplementary material for: 1D YIG hole-based magnonic nanocrystal
Source: arXiv:2506.10591 source file (2025-06-12)
Supplement: Supplementary file 1 [file SupMat.pdf]

"**1D YIG hole-based magnonic nanocrystal**" **<u>(SUPPLEMENTARY MATERIALS)</u>**

K. O. Levchenko[1], K. Davídková[1,2], R. O. Serha[1,2], M. Moalic[3], A. A. Voronov[1,2], C. Dubs[4], O. Surzhenko[4], M. Lindner[4], J. Panda[5], Q. Wang[6], O. Wojewoda[5], B. Heinz[7], M. Urbánek[5], M. Krawczyk[3], and A. V. Chumak[1]

[1)] *Faculty of Physics, University of Vienna, Vienna, Austria*

[2)] *Vienna Doctoral School in Physics, University of Vienna, Vienna, Austria*

[3)] *Department of Physics of Nanostructures, Adam Mickiewicz University, Poznań, Poland*

[4)] *INNOVENT e.V. Technologieentwicklung, Jena, Germany*

[5)] *CEITEC BUT, Brno University of Technology, Brno, Czech Republic*

[6)] *Institute for Quantum Science and Engineering, HUST, Wuhan, China*

[7)] *Fachbereich Physik & Landesforschungszentrum OPTIMAS, RPTU, Kaiserslautern, Germany*

## 1. Fabrication recipe

Considering the progress in material science and nanostructuring, the topic of magnonic crystals is making a swift comeback onto researchers' radar with, e.g., recently published works by Merbouche et al. [S1], on frequency filtering using width-modulated nanoscale Yttrium Iron Garnet (YIG) magnonic crystals (MCs), and by Mantion et al., who demonstrated reconfigurable spin-wave modes in a Heusler magnonic nanocrystal [S2]. Yet, the process of nanostructuring is complex and remains largely empirical, with no universal fabrication protocol. Currently, the limits of fabrication techniques define the minimum lateral size, which for us is around 50–100 nm for 100 nm-thick YIG films, increasing to around 300 nm for more complex periodic structures to guarantee repeatability and reliability.

To achieve the desired parameters of a 300 nm-wide MC waveguide periodically modulated with 150 nm-diameter holes along the entire conduit and considering 10 – 100 of such parallel waveguides on coplanar waveguide (CPW) antennas, our recipe included four main parts: fabrication of alignment markers, 'windows' at the position of the waveguides (using chromium as the hard mask, 'positive procedure'), fabrication of magnonic crystals (using CSAR as a hard mask, 'negative procedure'), and excitation antennas. Each part follows a similar set of steps: 1) cleaning and spin-coating (adhesion layer + resist CSAR for MC, PMMA – for rest + conductive layer ELECTRA); 2) electron beam writing of the target design (30 kV, 100 pA for MC and antennas, 9.23 nA for pads, labels, 'waveguides windows'); 3) developing (AR 600-546 for MC, AR 600-56 for the rest); 4) ion beam etching for MC or PMMA etch + evaporation + lift-off – for markers and antennas. After etching, the residual chromium mask was dissolved with Cr solvent. Microwave antennas were fabricated on top of MC conduits using e-beam lithography and electron-beam physical vapor deposition (10 nm Ti, 320 nm Cu, 20 nm Au).

To ensure optimal sampling control, each structure contains only one varying parameter, associated either with the magnonic crystal or distance between the antennas, and was replicated at different chip locations to minimize the impact of potential fabrication defects. The length of the waveguide was set to approximately 190 μm, based on preliminary estimation of the spin-wave propagation length in YIG thin films, ensuring that reflected spin waves from the waveguide edges do not interfere with the measurements. An alternative approach would be to use shorter waveguides while coating their ends with a thin gold layer to suppress backscattered signals [S3].

## 2. Antenna's excitation efficiency and dispersion relation calculation

In order to excite and detect spin waves in one-dimensional (1D) YIG MC periodically modulated with holes, each structure contained a pair of CPW antennas, spaced 1, 2, 5 and 10 μm apart. The antenna dimensions were optimized to maximize excitation efficiency and accessible wavenumber range, while also enabling the detection of multiple band gaps. Additionally, the design ensures operation at moderate microwave power levels, characteristic impedance $z_0 \approx 77\ \Omega$ for the excitation region and $z_0 \approx 50\ \Omega$ for the contact pads. Our previous experience with nanoscale YIG structures has shown that a reliable CPW antenna configuration has a ground-signal-ground (G-S-G) line layout, where the widths of the signal (S) and ground (G) lines are approximately 230 nm, and the gap between them is about 770 nm in the excitation region. The excitation efficiency of the CPW antenna is calculated based on the model proposed by Vlaminck et al., [S4], following the formula:

$$J_{\mathrm{exc}} = \left| \frac{2 \cdot \sin\left(\frac{k_t \cdot l_g}{2}\right)}{k_t \cdot l_g} + \frac{\sin\left(k_t \cdot \left(\frac{l_g}{2} + l_1\right)\right) - \sin\left(k_t \cdot \left(\frac{l_g}{2} + l_1 + l_p\right)\right)}{k_t \cdot l_p} \right|^2$$

where $l_g$ – width of a CPW signal line; $l_p$ – width of a CPW ground line; $l_1$ – distance between a signal and a ground line; $k_t$ – wavevector.

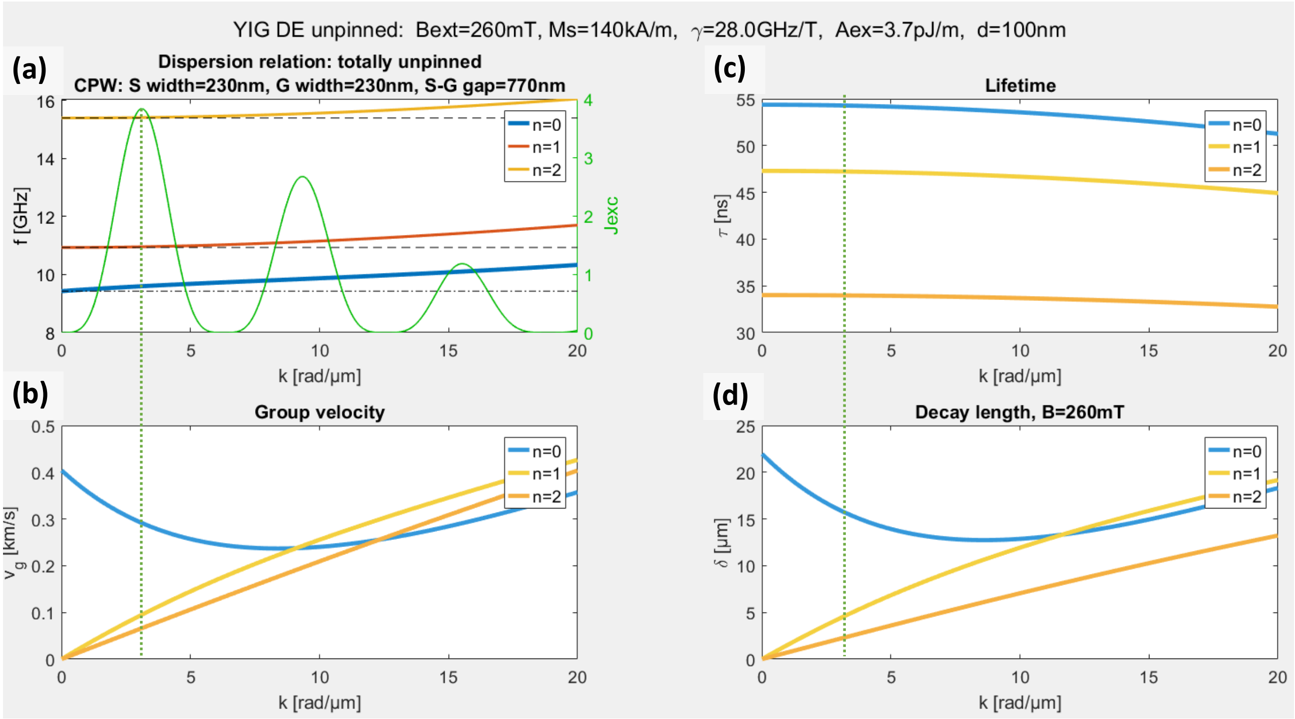


**Fig. S1:** Analytical calculation of the first three modes in 100 nm-thick YIG unstructured film ($M_s$ =176 mT, $\gamma$ = 28 GHz/T, $A_{ex}$ = 3.7 pJ/m) in Damon-Eshbach configuration under $\mu_0 H_{ext}$ = 260 mT bias field: **(a)** dispersion relation and CPW antenna's (ground-signal-ground, G-S-G, $w_{S,G} \approx$ 230 nm, $w_{S-G} \approx$ 770 nm) excitation efficiency $J_{exc}$; **(b)** group velocity $v_g$ (km/s); **(c)** lifetime $\tau$ (ns); **(d)** decay length $\delta$ (μm). Green dotted line represents a projection of a wavevector $k \approx 3.1 \frac{\mathrm{rad}}{\mu\mathrm{m}}$ corresponding to the lattice period of 1 μm.

The results of the analytical calculation of the dispersion relation for the first three spin-wave modes in an unstructured 100-nm-thick YIG film, together with the excitation efficiency $J_{exc}$ of the CPW antenna, are presented in Fig. S1**(a)**. We have considered standard magnetic parameter of the YIG film: $M_s$ = 176 mT, $\gamma$ = 28 GHz/T, $A_{ex}$ = 3.7 pJ/m, Damon-Eshbach (DE) configuration under the 260 mT bias magnetic field. In addition, we have also estimated the group velocity – $v_g$ (Fig. S1**(b)**), lifetime $\tau$ (Fig. S1**(c)**), decay length $\delta$ (Fig. S1**(d)**). According to Kalinikos and Slavin [S5, S6], the analytical description of the dipole-exchange spin waves in a ferromagnetic film considering the spin pinning condition is:

$$f = \frac{\gamma}{2\pi}\sqrt{\left(B_{ext} + \frac{2A_{ex}}{M_s}k^2\right)\left(B_{ext} + \frac{2A_{ex}}{M_s}k^2 + \mu_0 M_s F_n\right)},$$

where $k$ – total wavevector, $k = \sqrt{k_t^2 + k_n^2}$; $k_t$ – tangential wavevector, which corresponds to the spin-wave propagation in the magnetic film; $k_n = \frac{n\pi}{d}$ – perpendicular wavevector, which is quantized and defined by the film thickness $d$; $\mu_0$ –vacuum permeability; $\gamma$ –gyromagnetic ratio; $A_{ex}$ – exchange stiffness; $M_s$ – saturation magnetization; $B_{ext}$ – external magnetic field; $F_n$ – angular and boundary-condition-dependent term:

$$F_n = \sin^2\theta + P_n\left[\cos(2\theta) + \sin^2\theta \cdot \sin^2\phi \cdot \left(1 + \frac{\mu_0 M_s (1 - P_n)}{B_{ext} + \frac{2A_{ex}}{M_s}k^2}\right)\right],$$

where $\theta$ is an azimuthal angle, $\theta = \pi/2$ indicates in-plane magnetization; $\phi$ is the in-plane polar angle between the direction of spin-wave propagation and the direction of an effective field, $\phi = \pi/2$ corresponds

to wavevector perpendicular to magnetization, $P_n -$ spin-pinning condition term, which for unpinned magnetic moments is defined as:

$$P_n = \frac{k_t^2}{k^2}\left[1 - \frac{2k_t(1-(-1)^n e^{-k_t d})}{dk^2(1+\delta)}\right] \text{ with Kronecker's delta } \delta = \begin{cases} 1, & n = 0 \\ 0, & n \neq 0 \end{cases}.$$

Group velocity $v_{\mathrm{g}}$ was evaluated as a derivative of the dispersion relation:

$$v_{\mathrm{g}}(k_t) = \frac{d\omega}{dk} = 2\pi \cdot \frac{df_n}{dk} \approx 0.291 \text{ (km/s)},$$

where $f_n -$ frequency dispersions for the respective quantization number $n$ = 0, 1, 2,…; $\omega = 2\pi f -$ angular frequency.

Lifetime was calculated as a field derivative of the dispersion relation:

$$\tau = \left(\alpha\omega \frac{d\omega}{d\omega_{\mathrm{H}}}\right) \approx 54 \text{ (ns)},$$

where $\alpha -$ Gilbert damping constant.

Decay length was calculated according to:

$$\delta = v_{\mathrm{g}} \cdot \tau \approx 15.8 \text{ (µm)}.$$

Maximum excitation efficiency of the planned CPW antenna corresponds to $k \approx 3.1 \frac{\mathrm{rad}}{\mathrm{µm}} \rightarrow \lambda \approx$ 2 µm. The Bragg scattering condition of a 1D MC in the form of a periodic array of reflecting planes (holes) is defined as $n_{\mathrm{mc}}\lambda = 2a \sin\theta_{\mathrm{mc}}$, where $n_{\mathrm{mc}}$ is integer, $\lambda -$ spin-wave wavelength, $a$ – lattice constant (magnonic crystal period), $\theta_{\mathrm{mc}} -$ incident spin-wave angle. Assuming normal incidence ($\theta_{\mathrm{mc}} = \pi/2$), we set the MC period to $a = 1$ µm to achieve optimal excitation.

## 3. Micromagnetic simulations

### *3.1 TetraX mode profiles*

TetraX micromagnetic simulations were performed for the mode profiles in the DE and Backward Volume (BV) magnetization configuration of an unstructured waveguide cross-section considering (Fig. S2): $M_s$ = 174.7 mT, uniaxial magnetic anisotropy $K_{\mathrm{u}}$ = 3.58 J/m$^3$ (⊥ x-axis); Gilbert damping $\alpha = 10^{-4}$; waveguide's thickness $d$ = 100 nm; waveguide's width $\omega$ = 320 nm. Profiles were calculated for $k$ = 0, considering only the first five ($n$ = 5) modes due to the quadratic decrease in dynamic magnetization intensity with increasing $n$. The real part of the respective magnetization components – $m_y$ for DE, $m_x$ for BV – is color-coded with red and blue.

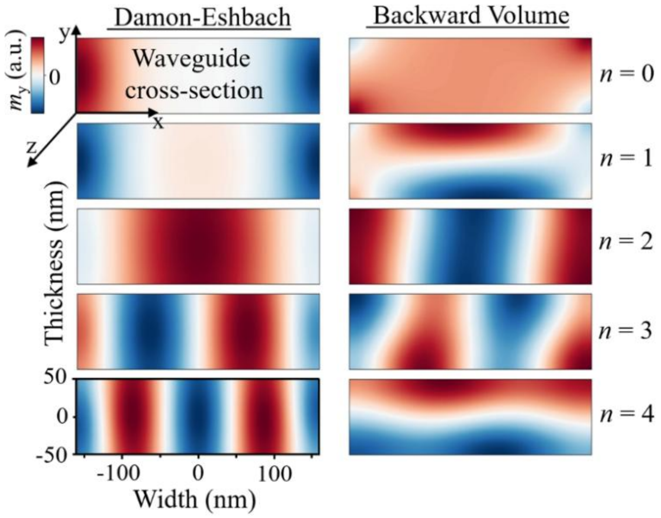


**Fig. S2**: TetraX simulation of the mode profile amplitudes for the first 5 spin-wave modes of the unstructured waveguide in DE and BV geometry.

Profiles exhibit both width and thickness quantization due to lateral confinement. In the DE configuration, all modes show only width quantization, with components $k_y = n\pi/w$, whereas the BV configuration displays a more complex mix of thickness and width contributions, evident from the horizontal and diagonal color patterns. The DE modes with $n = 0, 1$ are edge modes, where spin waves propagate only along the waveguide edges. Slight non-uniformities in the BV profiles, such as in the $n = 0$ mode, arises from plotting a single magnetization component, while contributions from both dynamic components $m_y$ and $m_x$ are

important. Although the mode profiles are unpinned at the top and bottom surfaces, edge pinning persists, introducing elastic scattering into higher-order width modes. This effect occurs because the waveguide width slightly exceeds the critical threshold required for complete unpinning and single-mode operation. The impact of edge pinning is more pronounced in DE modes due to their intrinsically nonreciprocal and edge-localized nature, which leads to mode anticrossing at lower wavevectors. Nevertheless, simulations confirm that for the selected MC waveguide geometry, the DE configuration provides the clearest understanding and control of spin-wave transmission.

### 3.2. *MuMax$^3$ dispersion relation of the 1D magnonic crystal waveguide*

The dispersion relation of the MC structure shown in Fig. 2**(b)** of the main article was calculated using Amumax, a fork of MuMax$^3$. The simulated geometry had parameters equal to those of the fabricated structures. The computational domain was discretized into 215 × 25 × 1 cells, corresponding to a spatial resolution of 6.1 × 10 × 100 nm along the x-, y-, and z-axes, respectively. The waveguide was modeled using YIG material parameters, with a saturation magnetization $M_\mathrm{s}$ = 174.7 mT, exchange stiffness $A_\mathrm{ex}$ = 3.7 $\cdot 10^{-12}$ J/m, and uniaxial magnetic anisotropy $K_\mathrm{u}$ = 3.58 J/m$^3$, oriented perpendicular to the x-axis. The Gilbert damping constant was set to $\alpha = 10^{-4}$. A static bias field of $B_\mathrm{ext}$ = 260 mT was applied along the y-axis. To break any residual symmetry that could lead to nonphysical results, additional static fields of 1 mT were applied along the x- and z-axes. Absorbing boundary conditions were implemented by gradually increasing the damping parameter near the edges of the waveguide.

The simulation proceeded in two stages. First, the system was relaxed to its magnetic ground state. Subsequently, spin waves were excited using a sinc-shaped magnetic field applied spatially, ensuring uniform excitation of wavevectors below $10^0 \times 10^6$ rad/m. The temporal profile of the excitation field also followed a sinc function, with a cut-off frequency of 15 GHz and a peak amplitude of $5 \times 10^{-4}$ T. The excitation was applied over a duration of 100 ns, and the x-component of the magnetization was sampled every 25.6 ps during this period. To compute the dispersion relation, the x-components of the magnetization were recorded as functions of time and position. A discrete Fourier transform was applied along both the time and x-axes using the fast Fourier transform (FFT) algorithm for each simulation cell. The absolute value of the resulting complex spectra was computed and summed over the z- and y-axes to yield the final dispersion map.

The spin-wave dispersion enabled the estimation of the relative positions of the band gaps within the magnonic spectrum and was in good agreement with TetraX dispersion calculation.

### 3.3. *TetraX simulations*

The dispersion relation as a function of the microwave frequency (Fig. 2**(c)** of the main article) was analytically calculated for a single unstructured MC conduit to match the experimental data. The calculations were performed using an open-source TetraX-based software, developed within the Nanomagnetism and Magnonics group by A. A. Voronov et al., at the University of Vienna (https://www.madivie.at/). Common input parameters for all calculated structures were: Damon-Eschbach configuration, $B_\mathrm{ext}$ = 262 mT; waveguide of width $w$ = 320 nm, $t$ = 100 nm; $M_s$ = 174.7 mT; in-plane anisotropy $K_\mathrm{u}$ = 3.58 J/m$^3$; exchange constant $A_\mathrm{ex}$ = 3.7 $\cdot 10^{-12}$ J/m; Gilbert damping $\alpha = 2 \cdot 10^{-4}$; wavevector range $k$ = 0...20 rad/µm; number of $k$-values = 100; mash cell size $dx, dy$ = 5, number of modes $n$ = 5.

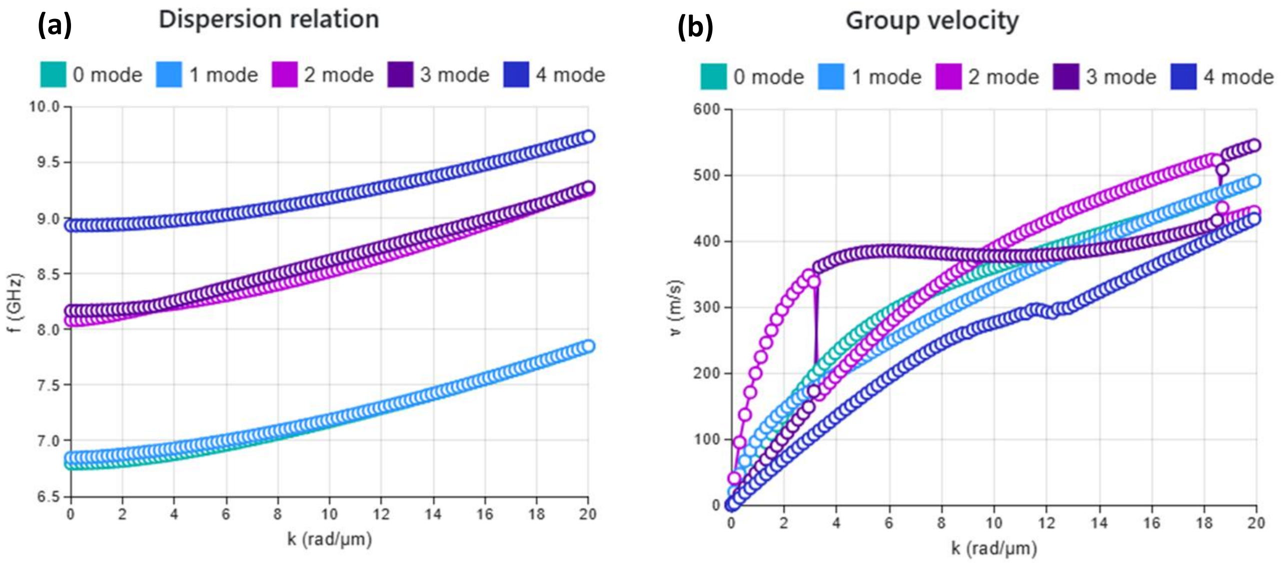

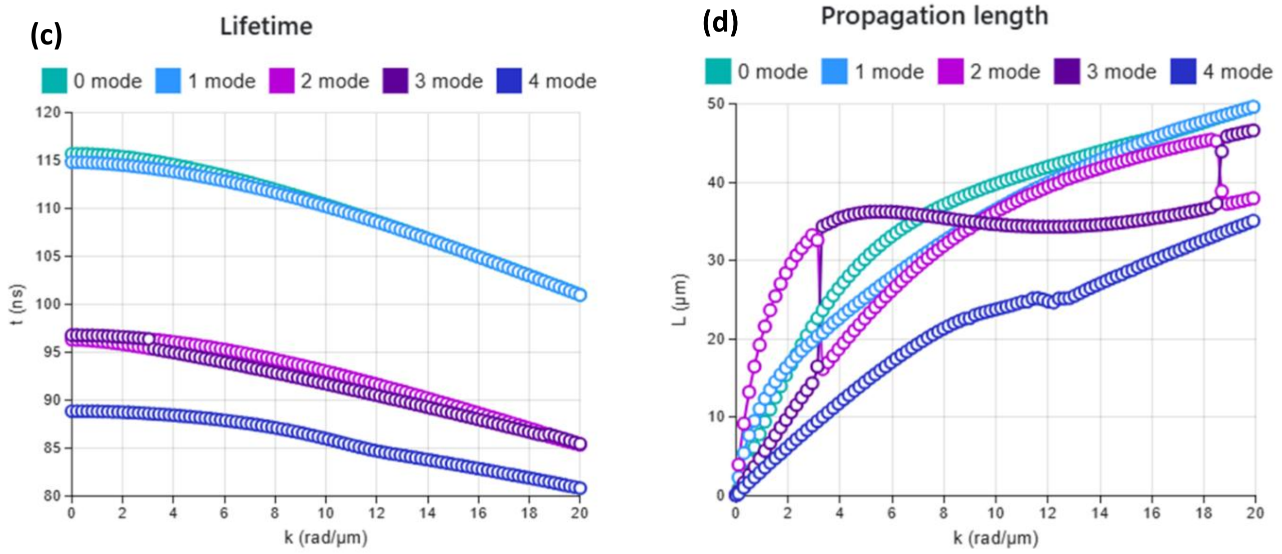


**Fig. S3**: TetraX micromagnetic simulation of the unstructured waveguide with a width $w = 320$ nm, thickness $t = 100$ nm, saturation magnetization $M_s = 174.7$ mT, and external magnetic field $\mu_0 H_{ext} = 262$ mT for the $n = 5$ modes: **(a)** spin-wave dispersion relation; **(b)** group velocity; **(c)** lifetime; **(d)** propagation length.

Notably, in the main article, only the modes $n = 2$ and 3 of the unstructured waveguide are shown with **crimson solid** and **peach dotted** lines respectively. In the Supplementary (Fig. S3), all 5 modes are shown in colors according to the program's default palette, with modes 2 and 3 represented with **purple** and **plum** circles, as noted in the figures' legend. First two modes correspond to the edge states, while the lowest fundamental width mode is $n = 2$. The derived parameters for the second mode around $k \approx 3.1$ rad/μm are estimated as: group velocity $v_g \approx 340$ m/s (Fig. S3**(b)**), lifetime $\tau \approx 95.9$ ns (Fig. S3**(c)**), propagation length $l \approx 32.7$ μm (Fig. S3**(d)**). At the $k \approx 3.1$ rad/μm and 18.7 rad/μm spin waves modes $n = 2$ and $n = 3$ are hybridized, forming anticrossing points, where energy is exchanged between the modes.

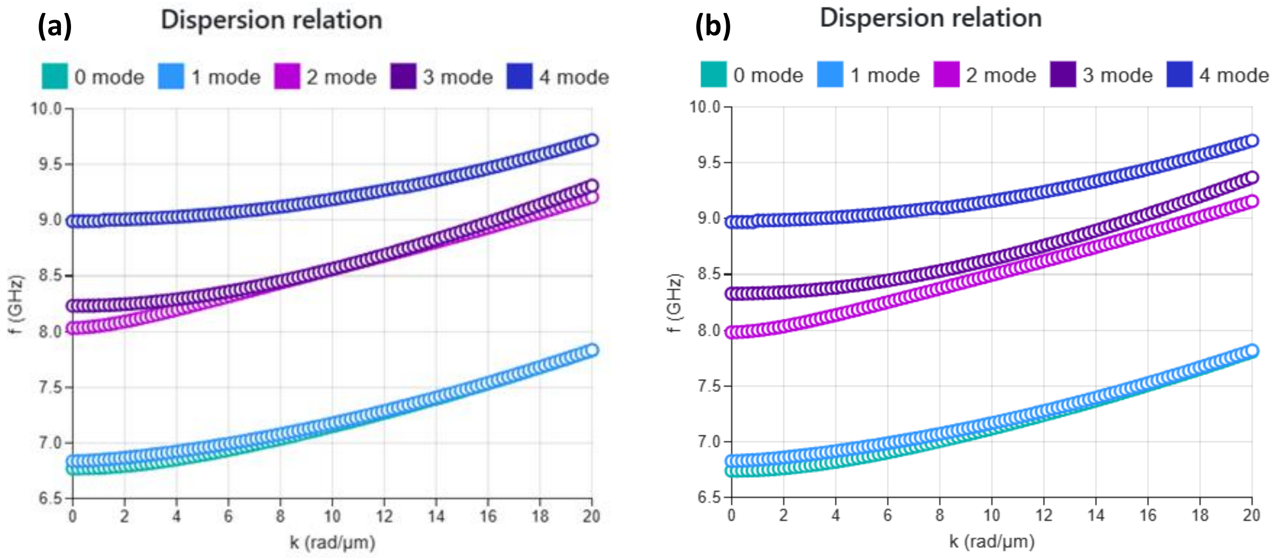

**(c)**

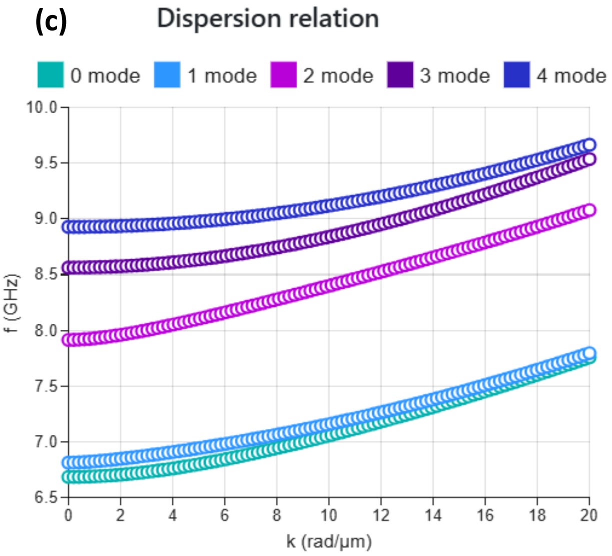


**Fig. S4**: TetraX micromagnetic simulations of the dispersion relations of an unstructured waveguide with parameters as in Fig. S3, varying in width: **(a)** width $w = 300$ nm; **(b)** width $w = 280$ nm; **(c)** width $w = 250$ nm.

Comparing Fig. S1 to Fig. S3 it is clearly visible how the much the dispersion relation of a thin film differs from the unstructured nanowaveguide. Firstly, a magnon frequency decreases in a waveguide under similar external magnetic field is primarily due to demagnetization field and mode confinement, which alters the effective internal field and dispersion relation. For discussed waveguide's configuration, mode localization ($n$ =2, 3) leads to two anticrossing points – at $k \approx 3.1$ rad/μm and $k \approx 18.7$ rad/μm. Therefore, a single-mode is expected within the frequency bandwidth of 100 MHz ($f \sim 8.08 - 8.17$ GHz, $k < 3.1$ rad/μm). Secondly, tuning of the geometrical parameters of the conduit, primary its width, most prominently affects the shape of the dispersion and modes hybridization.

For example, Fig. S4**(a)** shows the TetraX simulations of the dispersion relation for the waveguide with the same input parameters apart from the width set to originally designed 300 nm, while Fig. S4**(b)** and **(c)** – width set to 280 nm and 250 nm, respectively. It is clearly visible how the decrease of the width to 300 nm leads to the appearance of only 1 anticrossing point at $k \approx 8..11$ rad/μm, increasing the single-mode bandwidth to 200 MHz (8.03 – 8.23 GHz). Reducing the waveguide width to approximately 280 nm eliminates mode anticrossings, while further narrowing to 250 nm expands the single-mode frequency range sevenfold to 7.91 – 8.56 GHz (up to 12 rad/μm). A wider single-mode frequency bandwidth for the original structure is accessible in Backward Volume configuration – from 10.27 GHz to 10.94 GHz for the same input parameters (see Fig. S5). However, the excitation efficiency in such configuration was too low for measurement consideration.

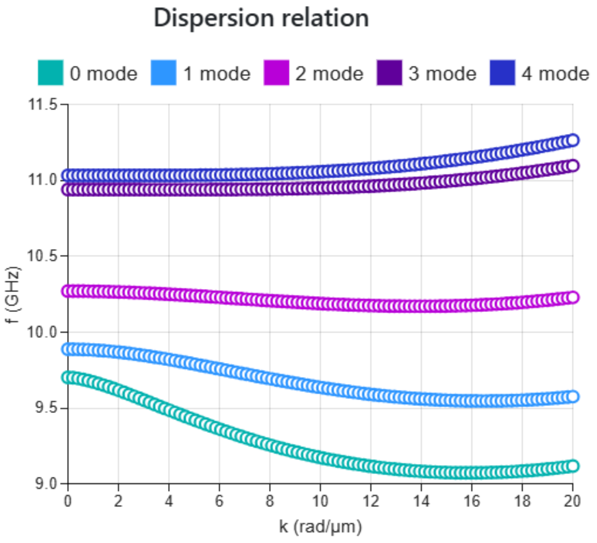


**Fig. S5**: TetraX micromagnetic simulation of the dispersion relation for an unstructured waveguide with the same parameters as in Fig. S3, but in the Backward Volume geometry.

## 4. Propagating spin-wave spectroscopy experimental set-up

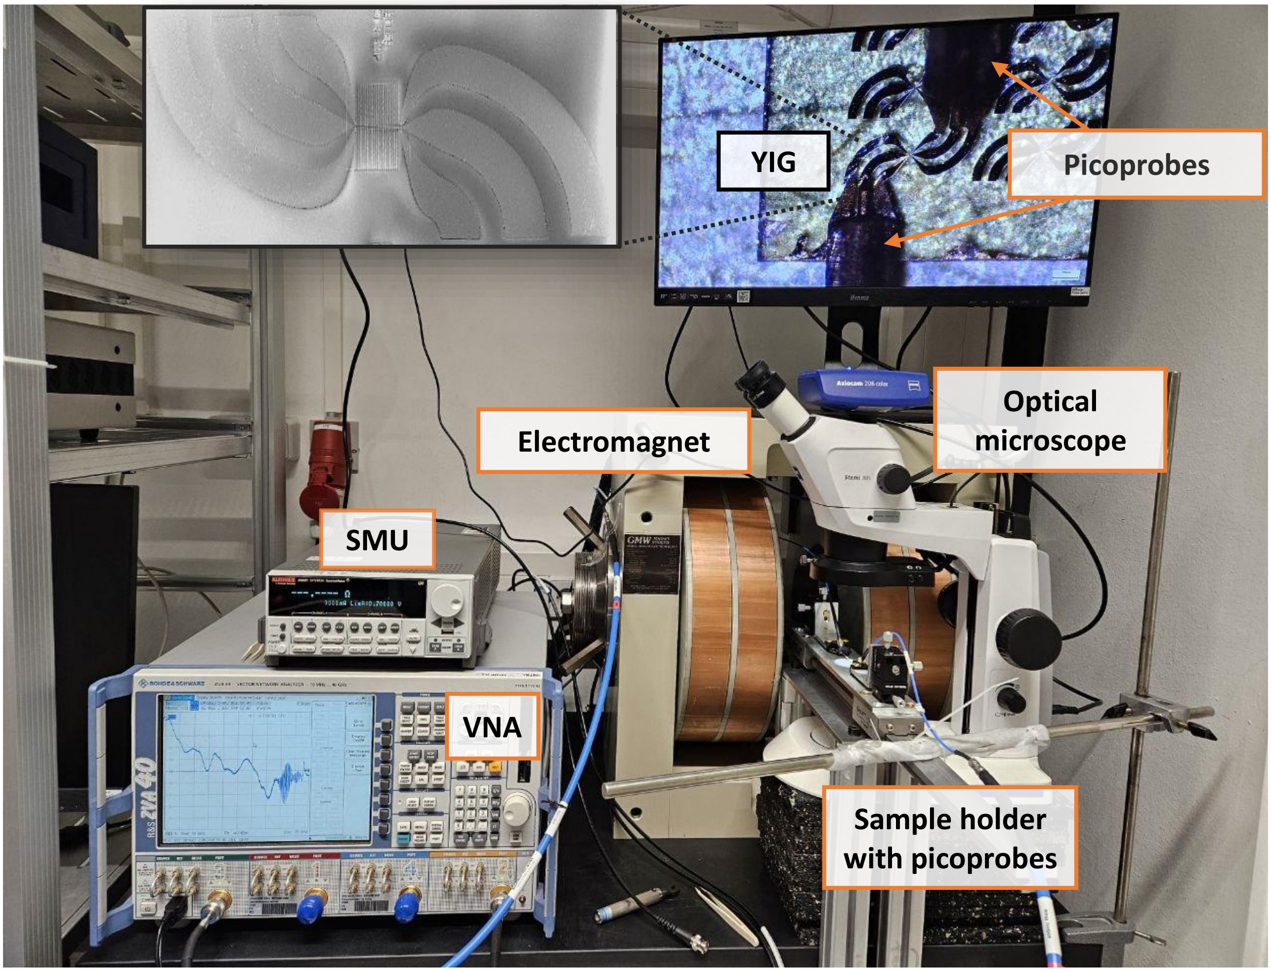


**Fig. S6**: Experimental setup used in propagating spin-wave spectroscopy (PSWS) measurements, consisting of key equipment: Vector Network Analyzer (VNA), coaxial k-type cables and adapters, 40A-GSG-150-P picoprobes, GMW 3473-70 electromagnet, Source Measurement Unit (SMU) and optical microscope.

All-electrical propagating spin-wave spectroscopy (PSWS) measurements were carried in the set-up shown in Fig. S6. The set-up consists of a Vector Network Analyzer, VNA (4-port Rhode & Schwarz ZVA-40) connected to an H-frame electromagnet GMW 3473-70 with a tunable air gap for various measurement configurations and magnet poles of 15 cm diameter to induce a sufficiently uniform biasing magnetic field ($\mu_0 H_{\mathrm{ext}} =$ <0.6…2.1 T depending on the air gap). The calibrated VNA signal was transferred via k-type cables/non-magnetic adapters to a pair of 40A-GSG-150-P picoprobes connected to the contact pads of the fabricated CPW antennas. All the measurements were performed at $T_{\mathrm{RT}} \approx 295\,K$. To avoid non-linear contributions from multimagnon scattering processes, preserve the antennas during extended measurements, yet achieve an optimal signal efficiency, we kept the RF power at -10 dBm. Sample is located between the picoprobes on a sample holder, and can be rotated with respect to the required magnetization geometry.

After applying sufficient magnetic field to homogenously magnetize the sample, VNA-generated high-frequency signal is transferred to a CPW antenna fabricated on top of the structure of interest. The applied microwave signal induces an alternating Oersted magnetic field around the antenna. Its components perpendicular to the bias field provide the necessary torque to excite precessional motion of spins in the magnetic medium directly under the antenna. If the correct conditions for the bias magnetic field and frequency are satisfied, this excitation launches propagating spin waves. By symmetry, the spin-wave detection mechanism through the output antenna is the inverse of the excitation. The VNA measures the transmitted and reflected signals, enabling the extraction of key parameters of transmission spectra, such as insertion loss, electromagnetic leakage, attenuation level, etc. VNA parameters used for the measurements were an intermediate frequency bandwidth 0.1-1 kHz, a frequency step 100 kHz and no averaging. Proper connection of picoprobes to sample's contact pads and evaluation of antennas' resistance was done via the Source Measurement Unit (SMU).

## 5. PSWS – different frequency ranges and ‘time gating’ for signal-to-noise improvement

Propagating spin-wave spectroscopy transmission signal $S_{12}$ of 100 nm-thick 1D YIG hole-based MC is shown on Fig. S7. The structure under study is same as demonstrated at Fig.1**(c)** of the main article and was measured under same conditions (Damon-Eshbach configuration; microwave signal power level set to -10 dBm). The reference background signal, taken at magnetic fields slightly below the excitation level, was subtracted to improve the signal-to-noise ratio. Most clear signal is demonstrated at Fig. S7**(b)** due to the optimal combination of the preliminary designed antenna’s excitation efficiency and high spin-wave group velocity.

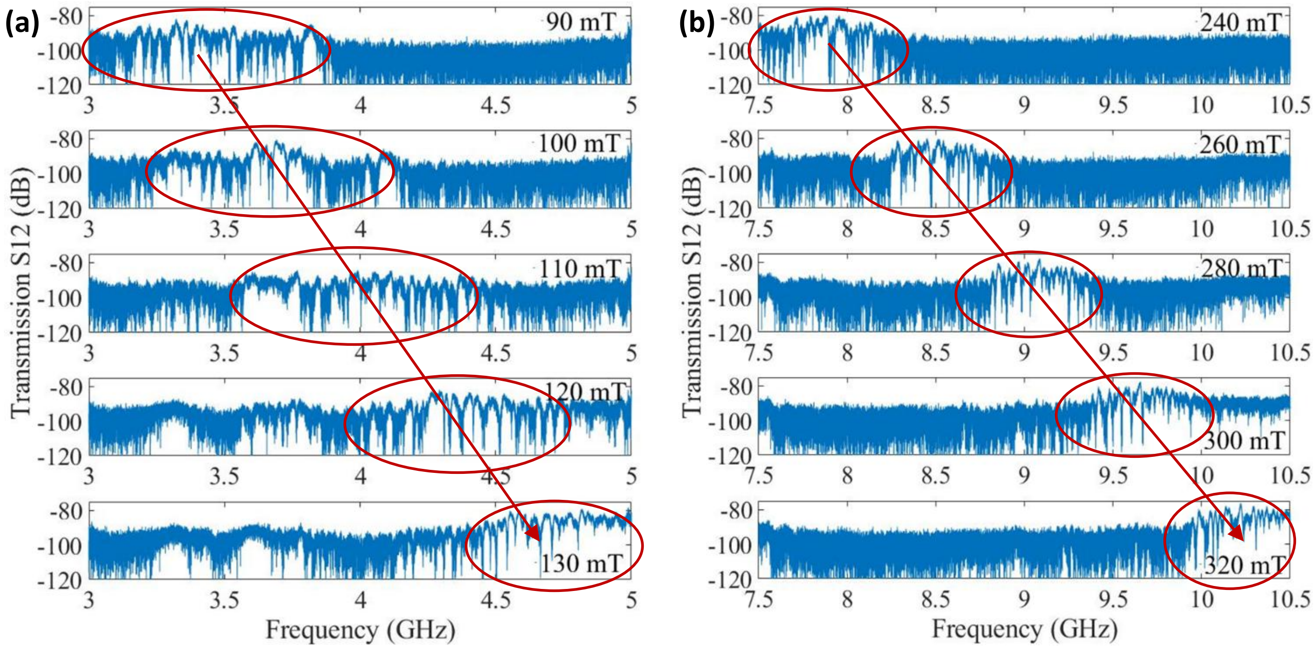


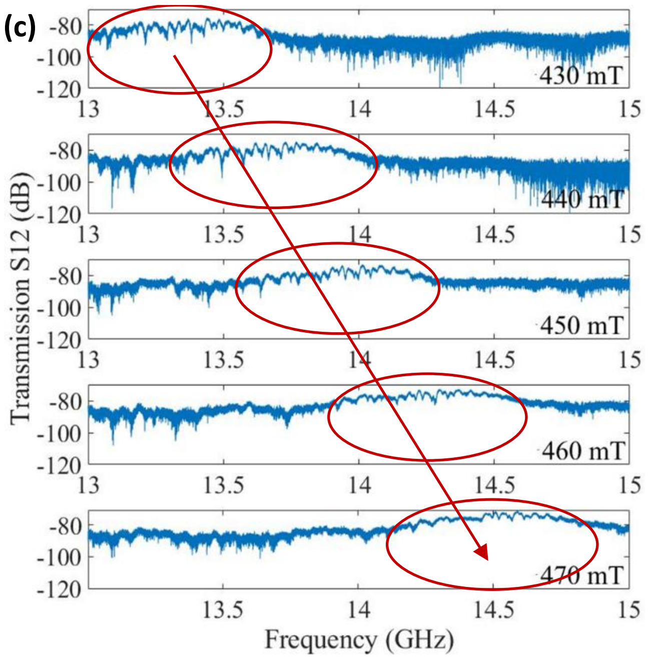


**Fig. S7**: Spin-wave transmission signal $S_{12}$ of 1D YIG hole-based MC (demonstrated at Fig. 1**(c)** of the main article) at varying bias magnetic fields corresponding to different frequency ranges: **(a)** 90…130 mT → 3…5 GHz; **(b)** 240…320 mT → 7.5…10.5 GHz; **(c)** 430…470 mT → 13…15 GHz. Measurements performed via the all-electrical PSWS in DE configuration; signal power level set to -10 dBm.

To further improve the signal-to-noise ratio and subtract the electromagnetic leakage, we have used ‘time gating technique’, widely applied in Surface Acoustic Waves (SAW) analysis [S7, S8]. Firstly, the real and imaginary parts of the quasi-continuous $S_{12}$ VNA signal and its reference were respectively subtracted from each other before being subjected to Inverse FFT (IFFT) – Fig. S8**(a)**. A significant source of a signal disruption originates from electromagnetic leakage generated by the antenna itself, which propagates between the CPW antennas at a speed of light within a first nanosecond (up to 2 ns considering reflection-induced smearing), and is identified in the time domain as a first pulse of strong amplitude. The SW signal is expected to have a propagation time of around 14.7 ns, considering the ≈ 5 μm distance between the antennas and the

spin-wave velocity of ≈ 340 m/s (according to the TetraX simulations of the unstructured waveguide, *Section 3.3* of the Supplementary materials for the lowest fundamental volume mode $n = 2$ slightly below 3.1 rad/μm). This closely matches the second pulse found in the time-domain data, appearing at 13.6 ns. Therefore, a SW transmission window is further fixed to the time frame 13.6 ns – 90 ns, while setting the rest to zero, to eliminate the parasitic signal and noise. The obtained signal is then transformed back to the frequency domain via the FFT – Fig. S8**(b)**. Note, that we do not differentiate here between the pure SW transmission and reflected components, e.g., triple transit.

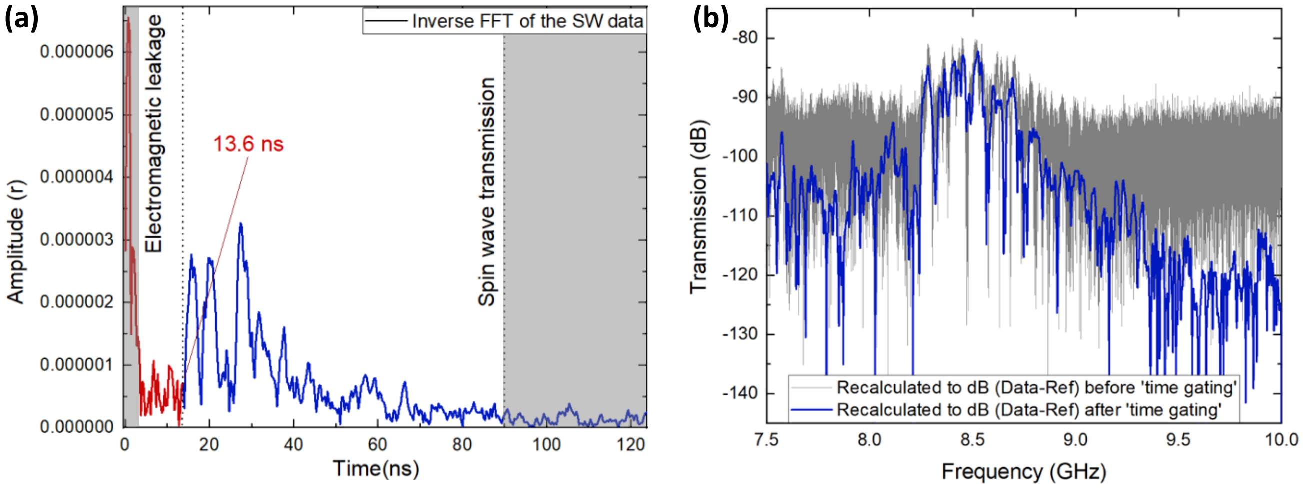


**Fig. S8**: Exemplary 'time gating' of the $S_{12}$ spin-wave transmission at a bias field of $\mu_0 H_{\text{ext}} = 260$ mT bias magnetic field: **(a)** Distinct peaks of spin-wave transmission and electromagnetic leakage in a time domain (inverse FFT from frequency domain); **(b)** Spin-wave transmission spectra (with a previously subtracted reference signal) before (gray) and after (blue) spurious signal removal. Time domain data in Fig. S3**(a)** conversed back to frequency domain via FFT.

## 6. PSWS at different power levels

All PSWS measurement discussed in the main article were performed at microwave power of -10 dBm. This value was identified as optimal based on a series of measurements at various VNA power levels, providing the best signal-to-noise ratio while maintaining operation within the linear regime (Fig. S9 **(a)**-**(f)** as indicated in the figures' top caption). Measurements performed on a structure of interest in Damon-Eshbach configuration, with no averaging of the signal and the intermediate frequency bandwidth set to 1 kHz.

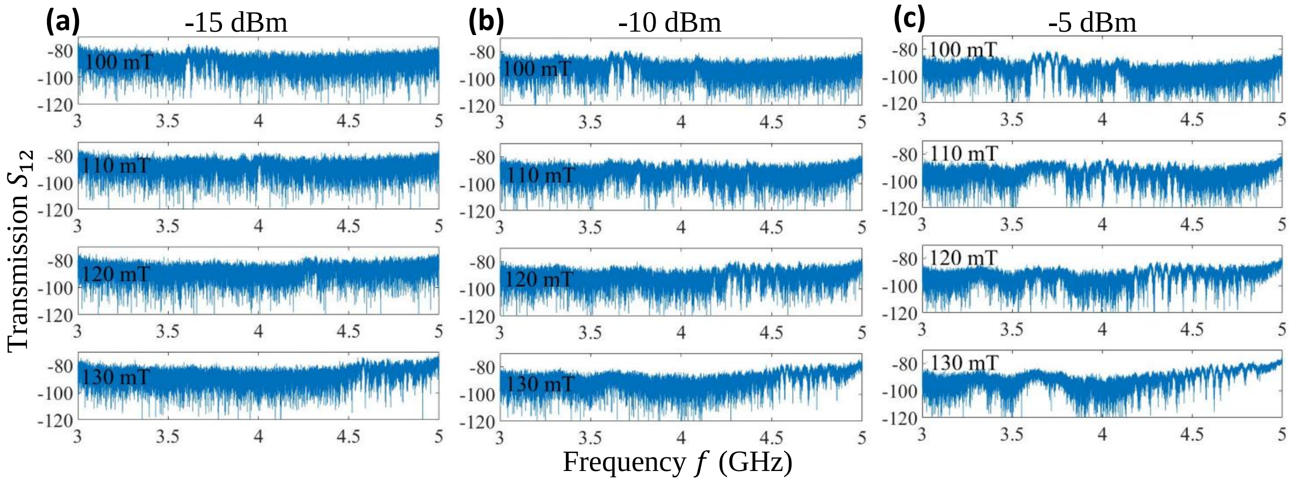

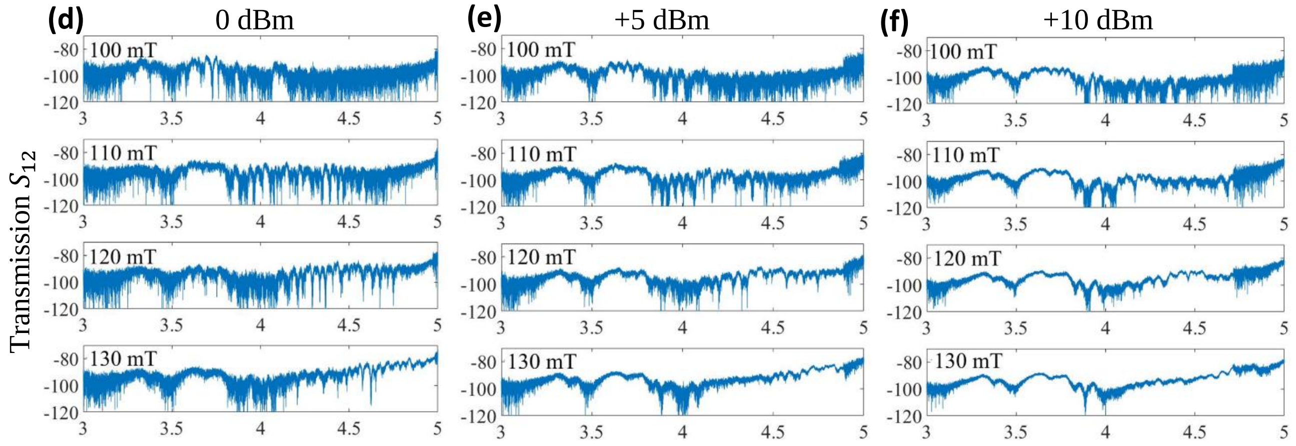


**Fig. S9**: Six $S_{12}$ transmission spectra of a structure of interest at six different microwave power levels each for four different external magnetic fields, as indicated in the figures.

## 7. μ-BLS frequency sweep

To study the spin-wave transmission in a single magnonic crystal, we have performed series of microfocused Brillouin light scattering spectroscopy (μ-BLS) measurements. μ-BLS is a crucial technique for current investigation as it provides spatially resolved spin-wave mapping of magnetization dynamics at the submicron scale, with a smallest distinguishable feature ≈ 300 nm. High resolution is achieved at a loss of $k$-resolution, as light is collected from multiple angles, leading to a mixture of different $k$-components in the detected signal. This is unlike $k$-resolved BLS, which uses a collimated laser beam at a defined angle of incidence to selectively probe certain wavevectors, but uses a large laser spot > 50 μm.

The measurements were performed on a different structure than the one used in PSWS analysis, as it was accidentally damaged. However, all relevant geometerical parameters remained the same (i.e., average waveguide's width and the holes' size), just the holes position were more centered. Distance between the antennas was ≈ 2 μm and number of conduits on antennas – 50, which were irrelevant for the BLS measurements.

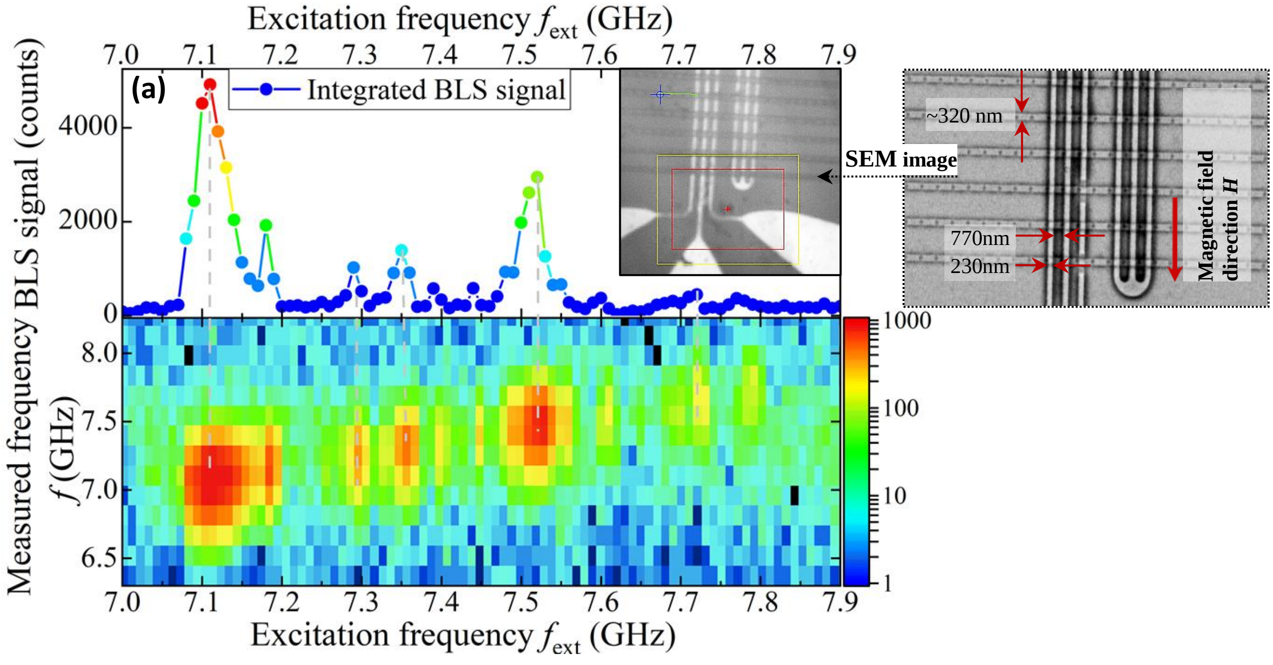

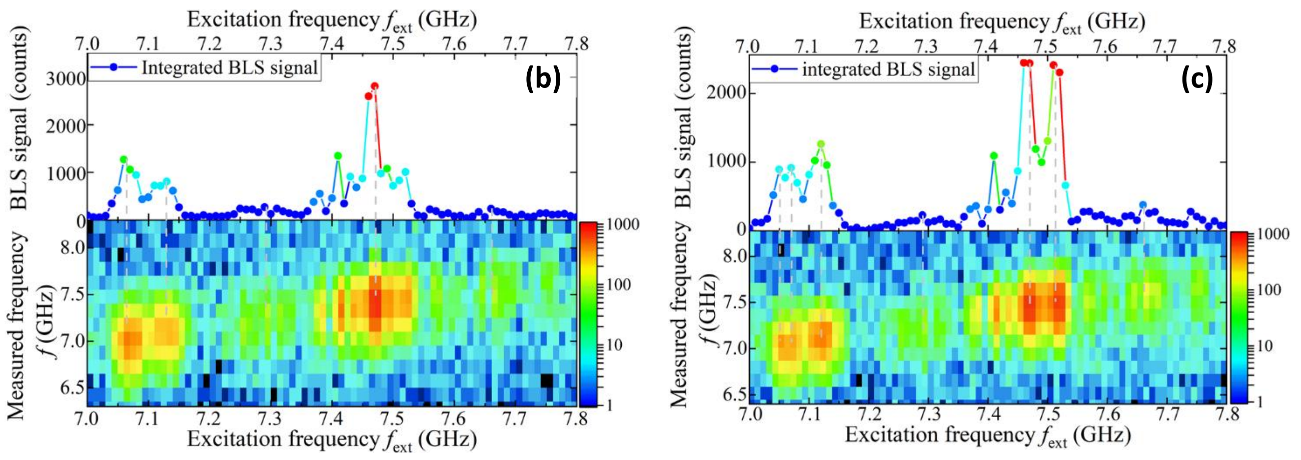


**Fig. S10**: BLS signal (detector counts) of the propagating spin wave as a function of a coherent excitation $f_{\text{ext}}$ (x-axis) in a form of: **(top section of each figure)** 2D graph, where each y-axis point corresponds to the integrated measured frequency $f$ over each respective excitation frequency $f_{\text{ext}}$; **(bottom section of each figure)** 3D intensity map (log scale), where the y-axis shows the full range of measured frequency $f$ at each excitation frequency $f_{\text{ext}}$, and BLS signal intensity is color-coded at z-axis. Three separate measurements **(a)** – **(c)** were performed at slightly shifted laser focus position along the short waveguide axis.

Firstly, we have performed the excitation frequency $f_{\text{ext}}$ sweep of a single magnonic crystal conduit at a fixed distance of ≈ 5 μm from coplanar waveguide, as shown at the set-up microscope's photo (Fig. S10**(a)**, inset) and schematically at the SEM image of the investigated structure (Fig. S10**(a)** right panel). The BLS laser was positioned in the middle of the MC waveguide. However, as the waveguide's dimensions are at the resolution limit of the microscope, three measurements (Fig. S10**(a)** – **(c)**) were performed with the same input parameters, but with the laser focus slightly shifted. It is clearly seen how the spin-wave propagation path from the excitation antenna to the detecting laser position is moderately changed, with passband frequency peaks displaying similar periodic pattern, but differ in their amplitude. Also, the spin-wave spectra shown in Fig. S10**(b)** and **(c)** are slightly downshifted in frequencies, as each measurement was taken separately with laser position set every time anew.

The first passband peak appeares around 7.05 GHz – 7.12 GHz with subsequent peaks spaced 0.19 GHz from each other (red-green areas on 3D maps). Regions dominated by the background BLS counts (blue areas on the 3D map) represent five band gaps measured 4.5 structural periods from the excitation antenna within a single MC waveguide. In patterned magnetic structures, inhomogeneous demagnetizing fields form at the edges of holes, locally modifying the internal magnetic field and leading to the localization of spin waves. These confined modes are highly sensitive to structural parameters such as hole size, spacing, and film thickness. As a result, fabrication imperfections—common in nanostructured thin films—can lead to variations in these parameters, contributing to the emergence of multiple peaks within one passband region, as well as changes to peaks' amplitude. Additionally, the generally lower signal intensity of propagating spin waves in thin films enhances the visibility of such parasitic modes.

Afterwards, we investigated the spin-wave transmission in the passband and band-gap regions by sweeping the laser position from 0 to 5 μm away from the antenna in around 100 nm step. Note, that Fig. S11 demonstrates the maximum BLS intensity at the passband excitation frequency $f_{\text{ext}} = 7.04$ GHz (red circles) and at the band-gap frequency $f_{\text{ext}} = 7.2$ GHz (blue squares), not integrated as in Fig. S10, for more clear representation. The passband signal is an order of magnitude stronger than that of a bandgap, confirming the SW filtering. Linear fitting reveals a smaller slope for the bandgap signal (light-blue dots) compared to the passband (orange dashes), indicating suboptimal excitation efficiency due to coarse excitation frequency choice, shifted starting position of the linescan from the vicinity of the antenna and enhanced signal dissipation due to holes directly beneath the antenna.

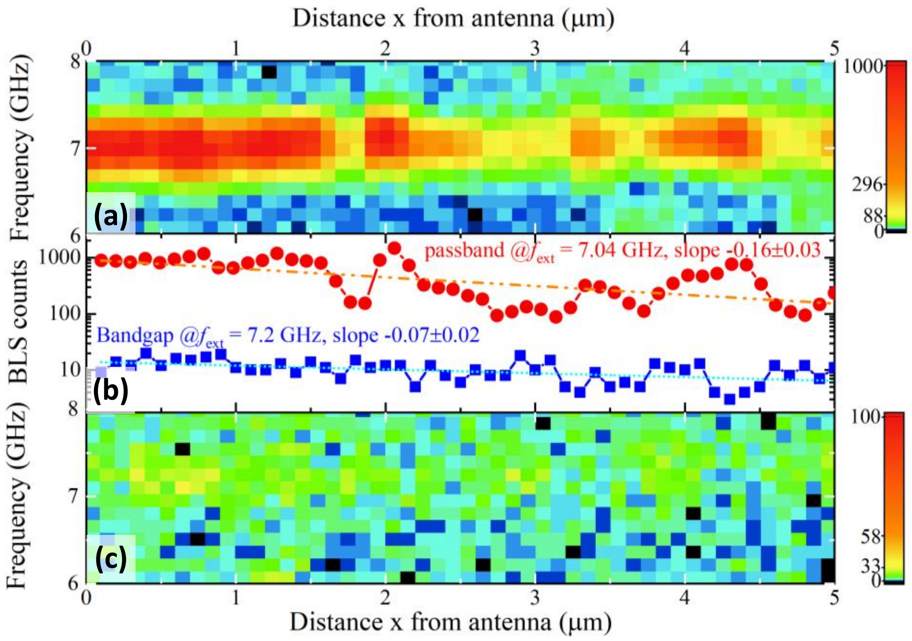


**Fig. S11**: BLS signal intensity of the propagating spin wave as a function of laser scan position 0-5 µm from the antenna (x-axis) in a form of: a 3D intensity map, where the y-axis shows the measured frequency $f$ at a passband **(a)** or band-gap **(c)** excitation frequencies $f_{\text{ext}}$, while the BLS signal intensity is color-coded on the z-axis; a 2D graph **(b)**, where each y-axis point corresponds to maximum BLS counts at the respective passband and band-gap frequencies.

## SUPPLEMENTARY MATERIALS LITERATURE:


[S1] H. Merbouche, et al., "Frequency Filtering with a Magnonic Crystal Based on Nanometer-Thick Yttrium Iron Garnet Films" *ACS Appl. Nano Mat.*, **4**(1), 121–128 (2021). DOI: 10.1021/acsanm.0c02382

[S2] S. Mantion, et al., "Reconfigurable spin wave modes in a Heusler magnonic crystal" *J. Appl. Phys.* **135**(5), 053902 (2024). DOI: 10.1063/5.0189486.

[S3] N. Kanazawa, et al., "The role of Snell's law for a magnonic majority gate" *Sci. Rep*. **7**, 7898 (2017). DOI: 10.1038/s41598-017-08114-7.

[S4] V. Vlaminck and M. Bailleul "Spin-wave transduction at the submicrometer scale: Experiment and modeling" *Phys. Rev. B* **81**, 014425 (2010). DOI: 10.1103/PhysRevB.81.014425.

[S5] B. A. Kalinikos, et al., "The dipole-exchange spin wave spectrum for anisotropic ferromagnetic films with mixed exchange boundary conditions" *J. Phys.: Condens. Matter* **2**, 9861 (1990). DOI: 10.1088/0953-8984/2/49/012.

[S6] B. A. Kalinikos, and A. N. Slavin. "Theory of dipole-exchange spin wave spectrum for ferromagnetic films with mixed exchange boundary conditions" *Journal of Physics C: Solid State Physics* **19**(35), 7013 (1986). DOI: 10.1088/0022-3719/19/35/014.

[S7] C. Heeg "Spin mechanics at radio frequencies" Ph.D. diploma thesis, Technische Universität München (2010).

[S8] I. Zdru, F. Ciubotaru, C. Nastase, A. Florescu, A. A. Hamadeh, M. Geilen, A. Nicoloiu, G. Boldeiu, D. Vasilache, S. Iordanescu, et al., "Interaction of Acoustic Waves With Spin Waves Using a GHz Operating GaN/Si SAW Device With a Ni/NiFeSi Layer Between Its IDTs" *IEEE Transac. Ultras. Ferroelectr. Freq. Contr*. **72**(1), 30 (2025). DOI: 10.1109/TUFFC.2024.3463731.
